# Supplementary material for: Synthesis and Inpainting-Based MR-CT Registration for Image-Guided Thermal Ablation of Liver Tumors
Source: arXiv:1907.13020 source file (2019-07-30)
Supplement: Supplementary file 1 [file Supplementary298.tex]

\pdfoutput=2
\documentclass[runningheads]{llncs}
\usepackage{amsfonts}
\usepackage{graphicx}
% Used for displaying a sample figure. If possible, figure files should
% be included in EPS format.
%
\usepackage{amsmath}
\usepackage{dcolumn}
\usepackage{amssymb}
\usepackage{etoolbox}
\usepackage{multirow}
\usepackage[misc]{ifsym}
\usepackage{changes}
	\definechangesauthor[name={Per cusse}, color=orange]{per}
	\setremarkmarkup{(#2)}

\BeforeBeginEnvironment{figure}{\vskip-2ex}
\AfterEndEnvironment{figure}{\vskip-2ex}
\AfterEndEnvironment{table}{\vskip-1ex}
% If you use the hyperref package, please uncomment the following line
% to display URLs in blue roman font according to Springer's eBook style:
% \renewcommand\UrlFont{\color{blue}\rmfamily}

\begin{document}
\title{Synthesis and Inpainting-Based MR-CT Registration for Image-Guided Thermal Ablation of Liver Tumors: Supplementary Material}
%
%\titlerunning{Abbreviated paper title}
\titlerunning{Synthesis and Inpainting-Based MR-CT Registration for Thermal Ablation}
% If the paper title is too long for the running head, you can set
% an abbreviated paper title here
%
%\author{***}
%
%\authorrunning{F. Author et al.}
% First names are abbreviated in the running head.
% If there are more than two authors, 'et al.' is used.
%
%\institute{***}
\author{Dongming Wei\inst{1,2} \and Sahar Ahmad\inst{2} \and Jiayu Huo\inst{1} \and Wen Peng\inst{3} \and Yunhao Ge\inst{4}  \and Zhong Xue\inst{4} \and Pew-Thian Yap\inst{2} \and Wentao Li\inst{5} \and Dinggang Shen\inst{2}\textsuperscript{(\Letter)} \and Qian Wang\inst{1}\textsuperscript{(\Letter)}}
%index{Last Name, First Name}
%1{Wei, Dongming}
%2{Ahmad, Sahar}
%3{Huo, Jiayu}
%4{Peng, Wen}
%5{Ge, Yunhao}
%6{Xue, Zhong}
%7{Yap, Pew-Thian}
%8{Li, Wentao}
%9{Shen, Dinggang}
%10{Wang, Qian}
\authorrunning{D. Wei et al.}

\institute{Institute for Medical Imaging Technology, School of Biomedical Engineering,
Shanghai Jiao Tong University, Shanghai 200030, China\\ \email{wang.qian@sjtu.edu.cn}
\and Department of Radiology and Biomedical Research Imaging Center (BRIC), University of North Carolina
at Chapel Hill, Chapel Hill, NC 27599, USA\\
\email{dgshen@med.unc.edu}
\and North China Electric Power University, Beijing, China
\and Shanghai United Imaging Intelligence Co., Ltd, Shanghai, China
\and Shanghai Cancer Center, Fudan University, Shanghai, China
}
\maketitle              % typeset the header of the contribution

\begin{table}[h]
    \scriptsize
    \centering
    \caption{The layer configurations of UR-Net. Conv3D represents the 3D convolution layer with the specified filter size, stride and number of filters. The Padding column indicates whether the Conv3D followed by zero padding to keep feature map size same. Skip connection is shown using Concat, which concatenates the previous neareset neighbor upsampled feature map with the corresponding Conv3D's feature map.}
    \begin{tabular}{c|c|c|c|c|c}
    \hline \hline
         Layer Name & Filter Size & Number of Filter & Stride & Padding & Nonlinearity  \\ \hline
         Concat\_1(Moving, Fixed) & & & & & \\
         Conv3D\_1 & $3\times3\times3$ & 2 & 1 & Y & LeakyReLU(0.2) \\
         Conv3D\_2 & $3\times3\times3$ & 2 & 1 & Y & LeakyReLU(0.2) \\ 
         \hline
         Conv3D\_3 & $3\times3\times3$ & 16 & 2 & Y & LeakyReLU(0.2) \\
         Conv3D\_4 & $3\times3\times3$ & 32 & 1 & Y & LeakyReLU(0.2) \\
         \hline
         Conv3D\_5 & $3\times3\times3$ & 32 & 2 & Y & LeakyReLU(0.2) \\
         Conv3D\_6 & $3\times3\times3$ & 32 & 1 & Y & LeakyReLU(0.2) \\
         \hline
         Conv3D\_7 & $3\times3\times3$ & 32 & 2 & Y & LeakyReLU(0.2) \\
         Conv3D\_8 & $3\times3\times3$ & 32 & 1 & Y & LeakyReLU(0.2) \\
         \hline
         Conv3D\_9 & $3\times3\times3$ & 32 & 2 & Y & LeakyReLU(0.2) \\
         Conv3D\_10 & $3\times3\times3$ & 32 & 1 & Y & LeakyReLU(0.2) \\
         Conv3D\_11 & $3\times3\times3$ & 32 & 1 & Y & LeakyReLU(0.2) \\
         \hline
         Upsampling3D\_1 & & 32 & 2 &  & \\
         Concat\_2(Conv3D\_8) & & 32+32 & & & \\
         Conv3D\_12 & $3\times3\times3$ & 32 & 1 & Y & LeakyReLU(0.2) \\
         \hline
         Upsampling3D\_2 & & 32 & 2 &  & \\
         Concat\_3(Conv3D\_6) & & 32+32 & & & \\
         Conv3D\_13 & $3\times3\times3$ & 32 & 1 & Y & LeakyReLU(0.2) \\
         \hline
         Upsampling3D\_3 & & 32 & 2 &  & \\
         Concat\_4(Conv3D\_4) & & 32+32 & & & \\
         Conv3D\_14 & $3\times3\times3$ & 32 & 1 & Y & LeakyReLU(0.2) \\
         Conv3D\_15 & $3\times3\times3$ & 16 & 1 & Y & LeakyReLU(0.2) \\
         \hline
         Upsampling3D\_4 & & 16 & 2 &  & \\
         Concat\_4(Conv3D\_2) & & 2+16 & & & \\
         Conv3D\_16 & $3\times3\times3$ & 6 & 1 & Y & LeakyReLU(0.2) \\
         Conv3D\_17 & $3\times3\times3$ & 3 & 1 & Y & Linear \\
         \hline\hline
    \end{tabular}
    \label{tab:my_label}
\end{table}

\end{document}
